# Supplementary material for: Self-supervised 3D Representation Learning of Dressed Humans from Social Media Videos
Source: arXiv:2103.03319 source file (2022-12-27)
Supplement: Supplementary file 1 [file cvpr_supp_attached.tex]

\newpage

% \appendix 

\begin{figure*}[t]
\begin{center}
{\includegraphics[width=0.8\textwidth]{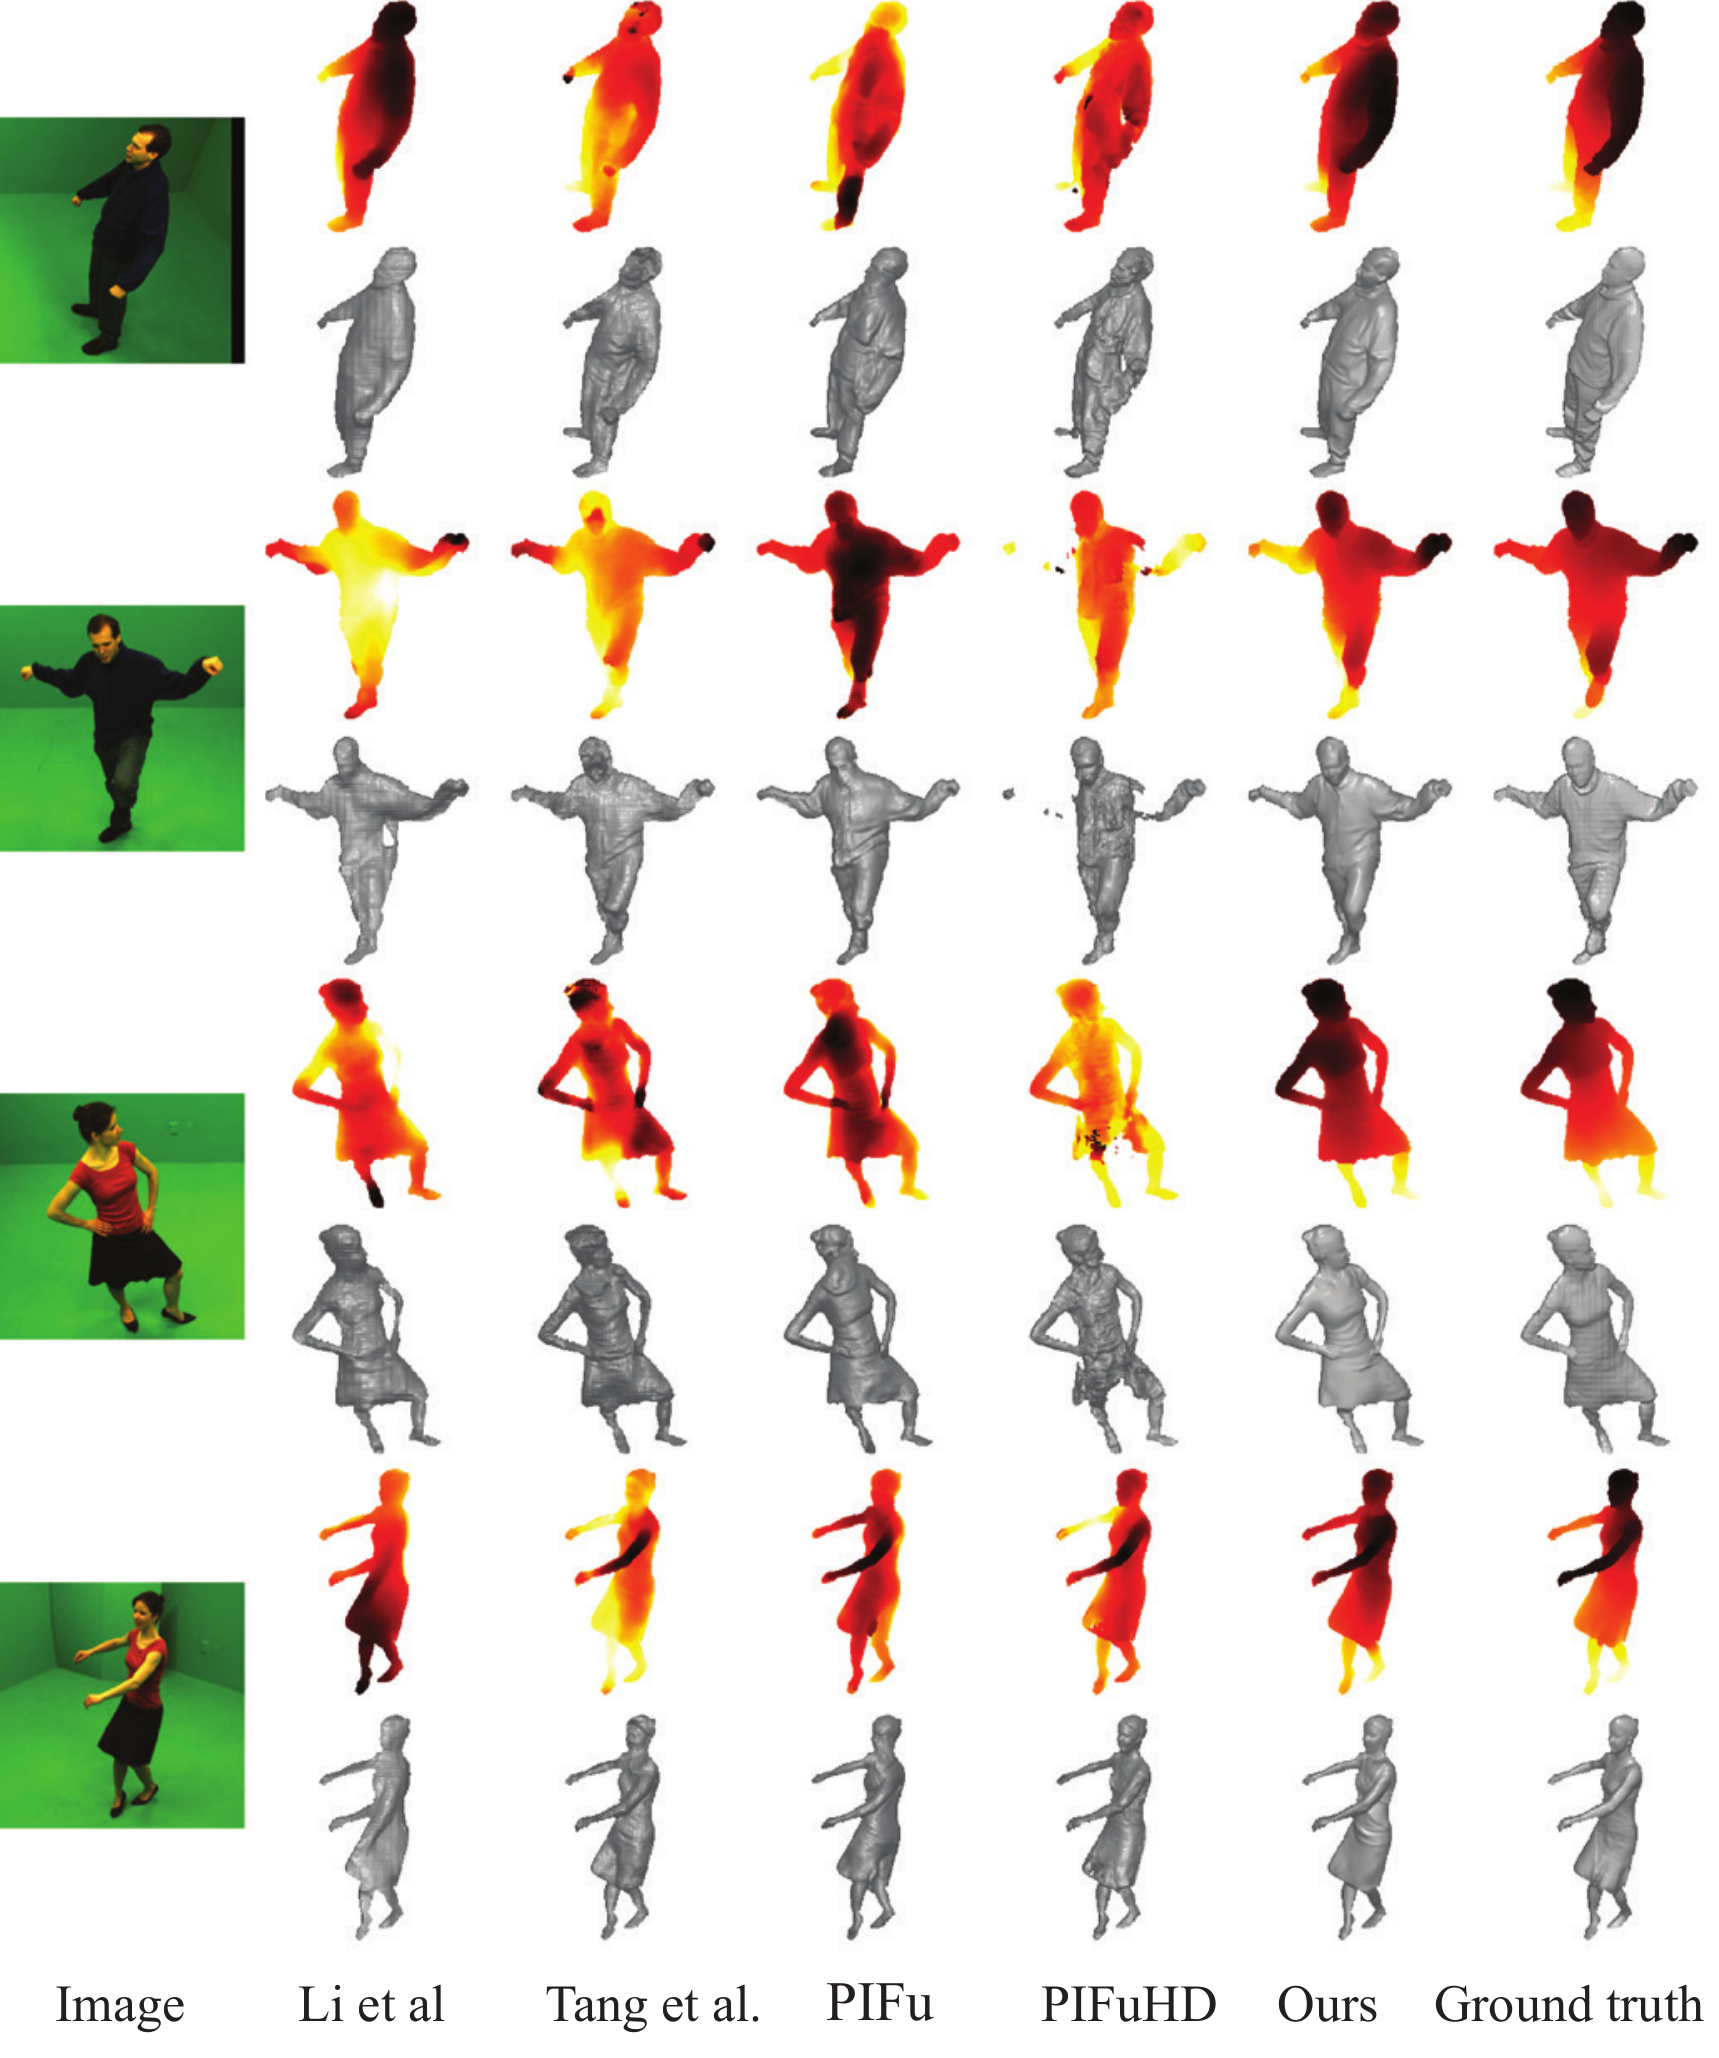}}
\end{center}
\vspace{-4mm}
    \caption{Qualitative comparison on Vlasic et al. dataset}
    \label{Fig:adobe1}
\end{figure*}

\begin{figure*}[t]
\begin{center}
{\includegraphics[width=0.8\textwidth]{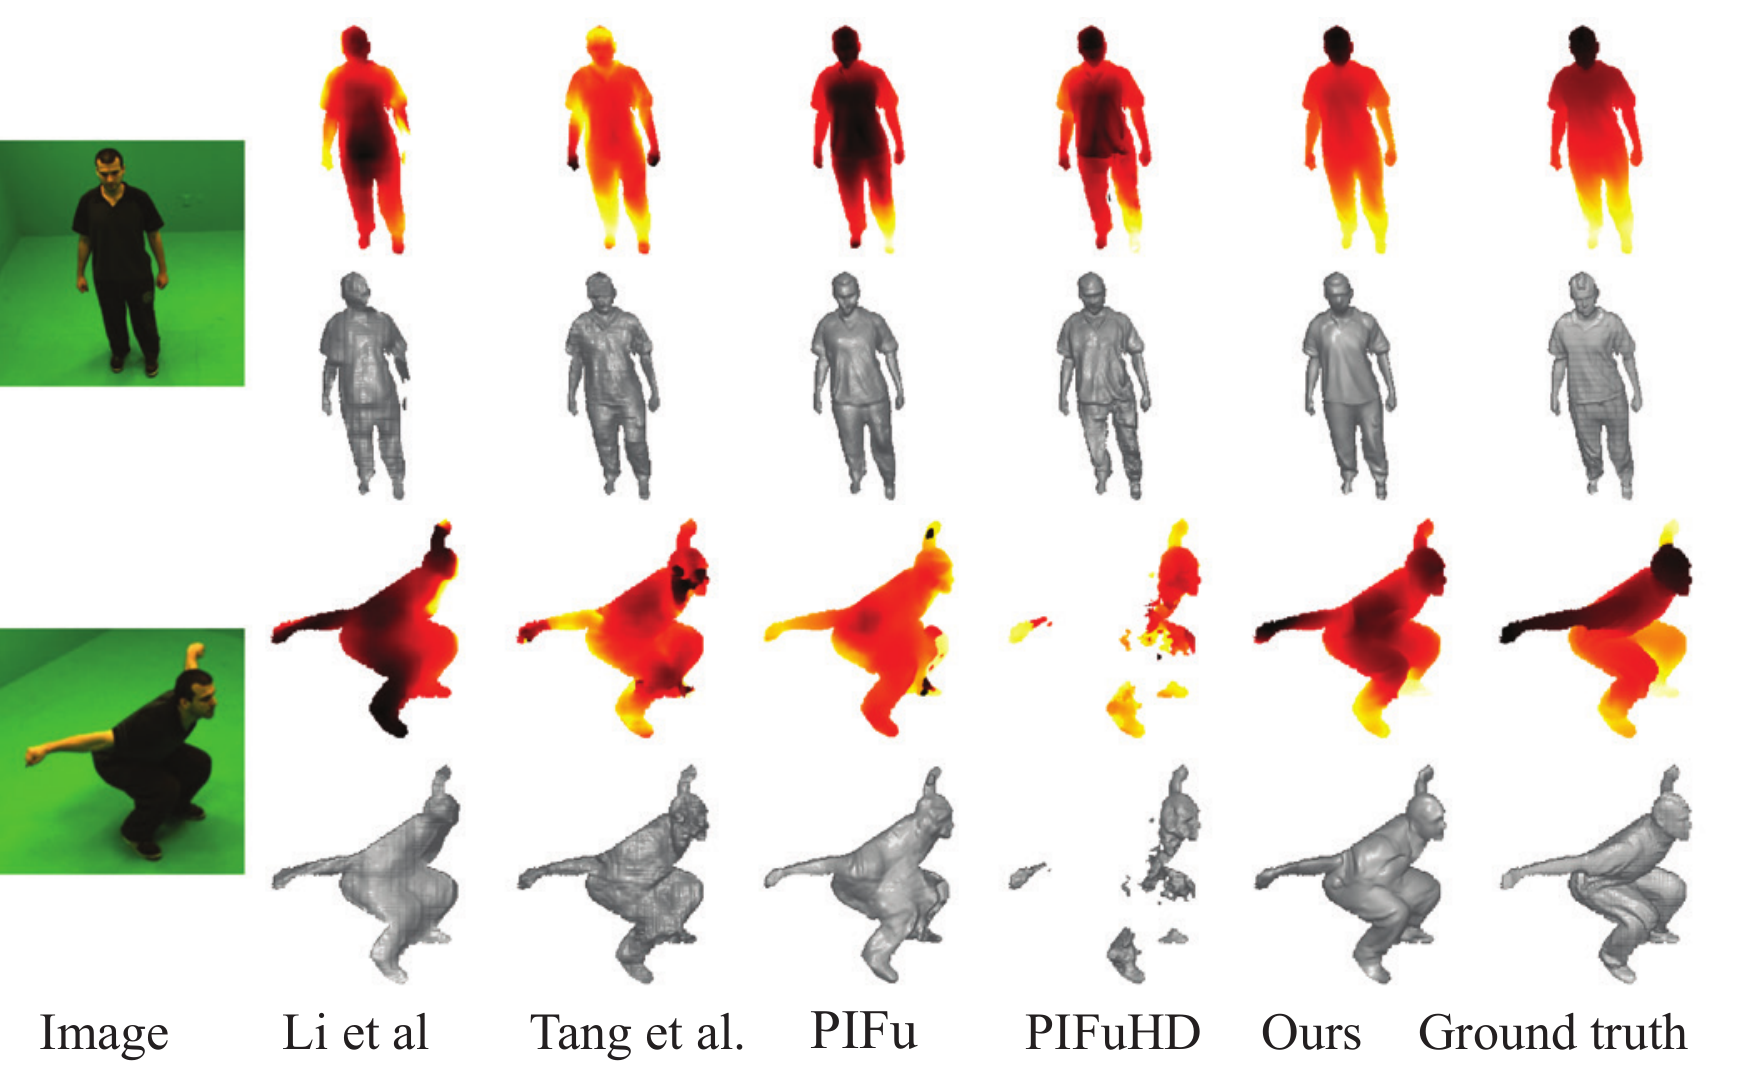}}
\end{center}
\vspace{-4mm}
   \caption{Qualitative comparison on Vlasic et al. dataset}
   \label{Fig:adobe2}
\end{figure*}

\begin{figure*}[t]
\begin{center}
{\includegraphics[width=0.8\textwidth]{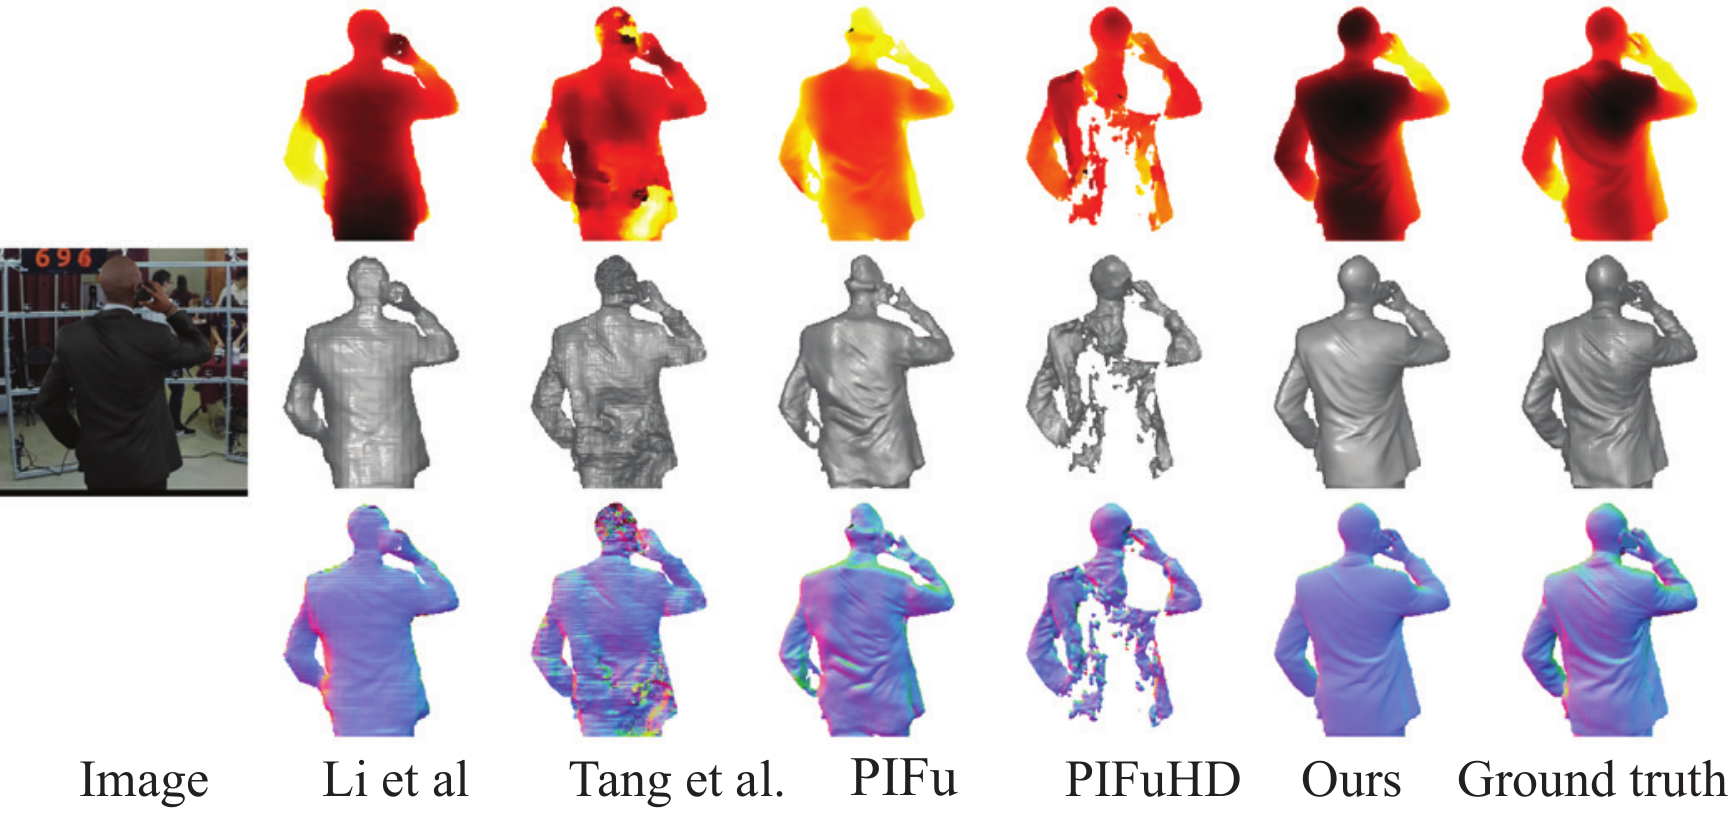}}
\end{center}
\vspace{-4mm}
   \caption{Qualitative comparison on RenderPeople testing dataset}
   \label{Fig:adobe3}
\end{figure*}

\begin{figure*}[t]
\begin{center}
{\includegraphics[width=0.8\textwidth]{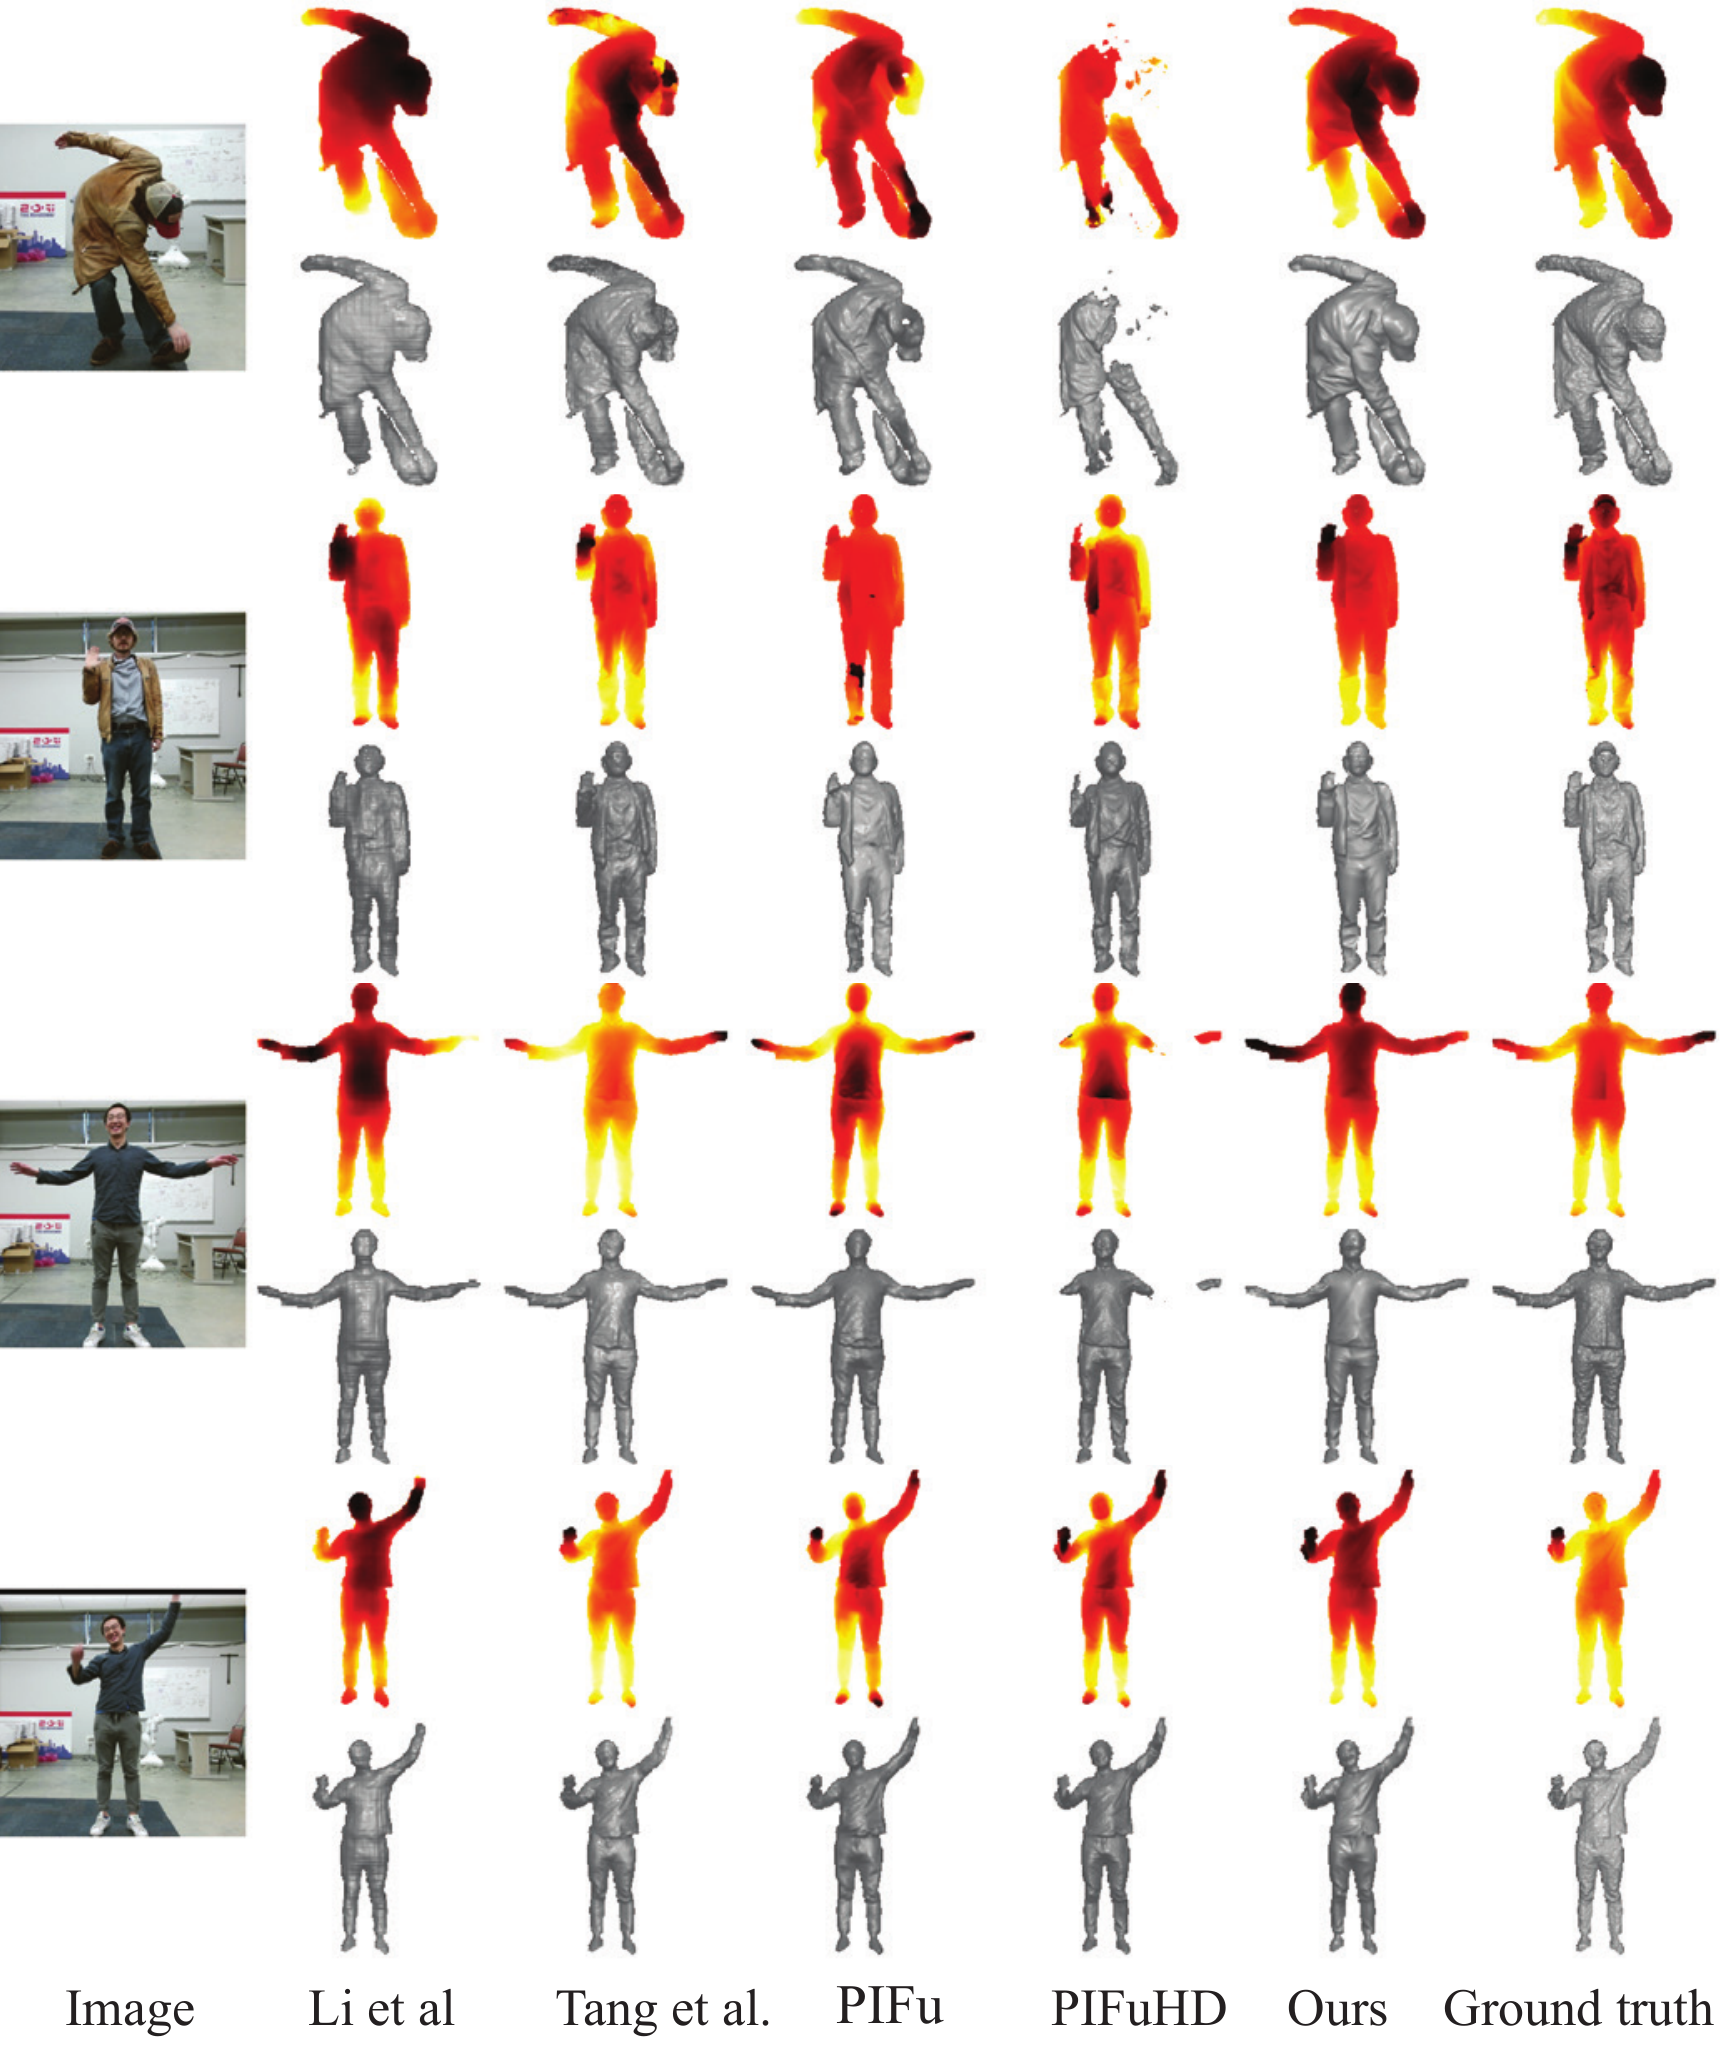}}
\end{center}
\vspace{-4mm}
   \caption{Qualitative comparison on Tang et al. training dataset}
   \label{Fig:adobe4}
\end{figure*}

\begin{figure*}[t]
\begin{center}
{\includegraphics[width=0.8\textwidth]{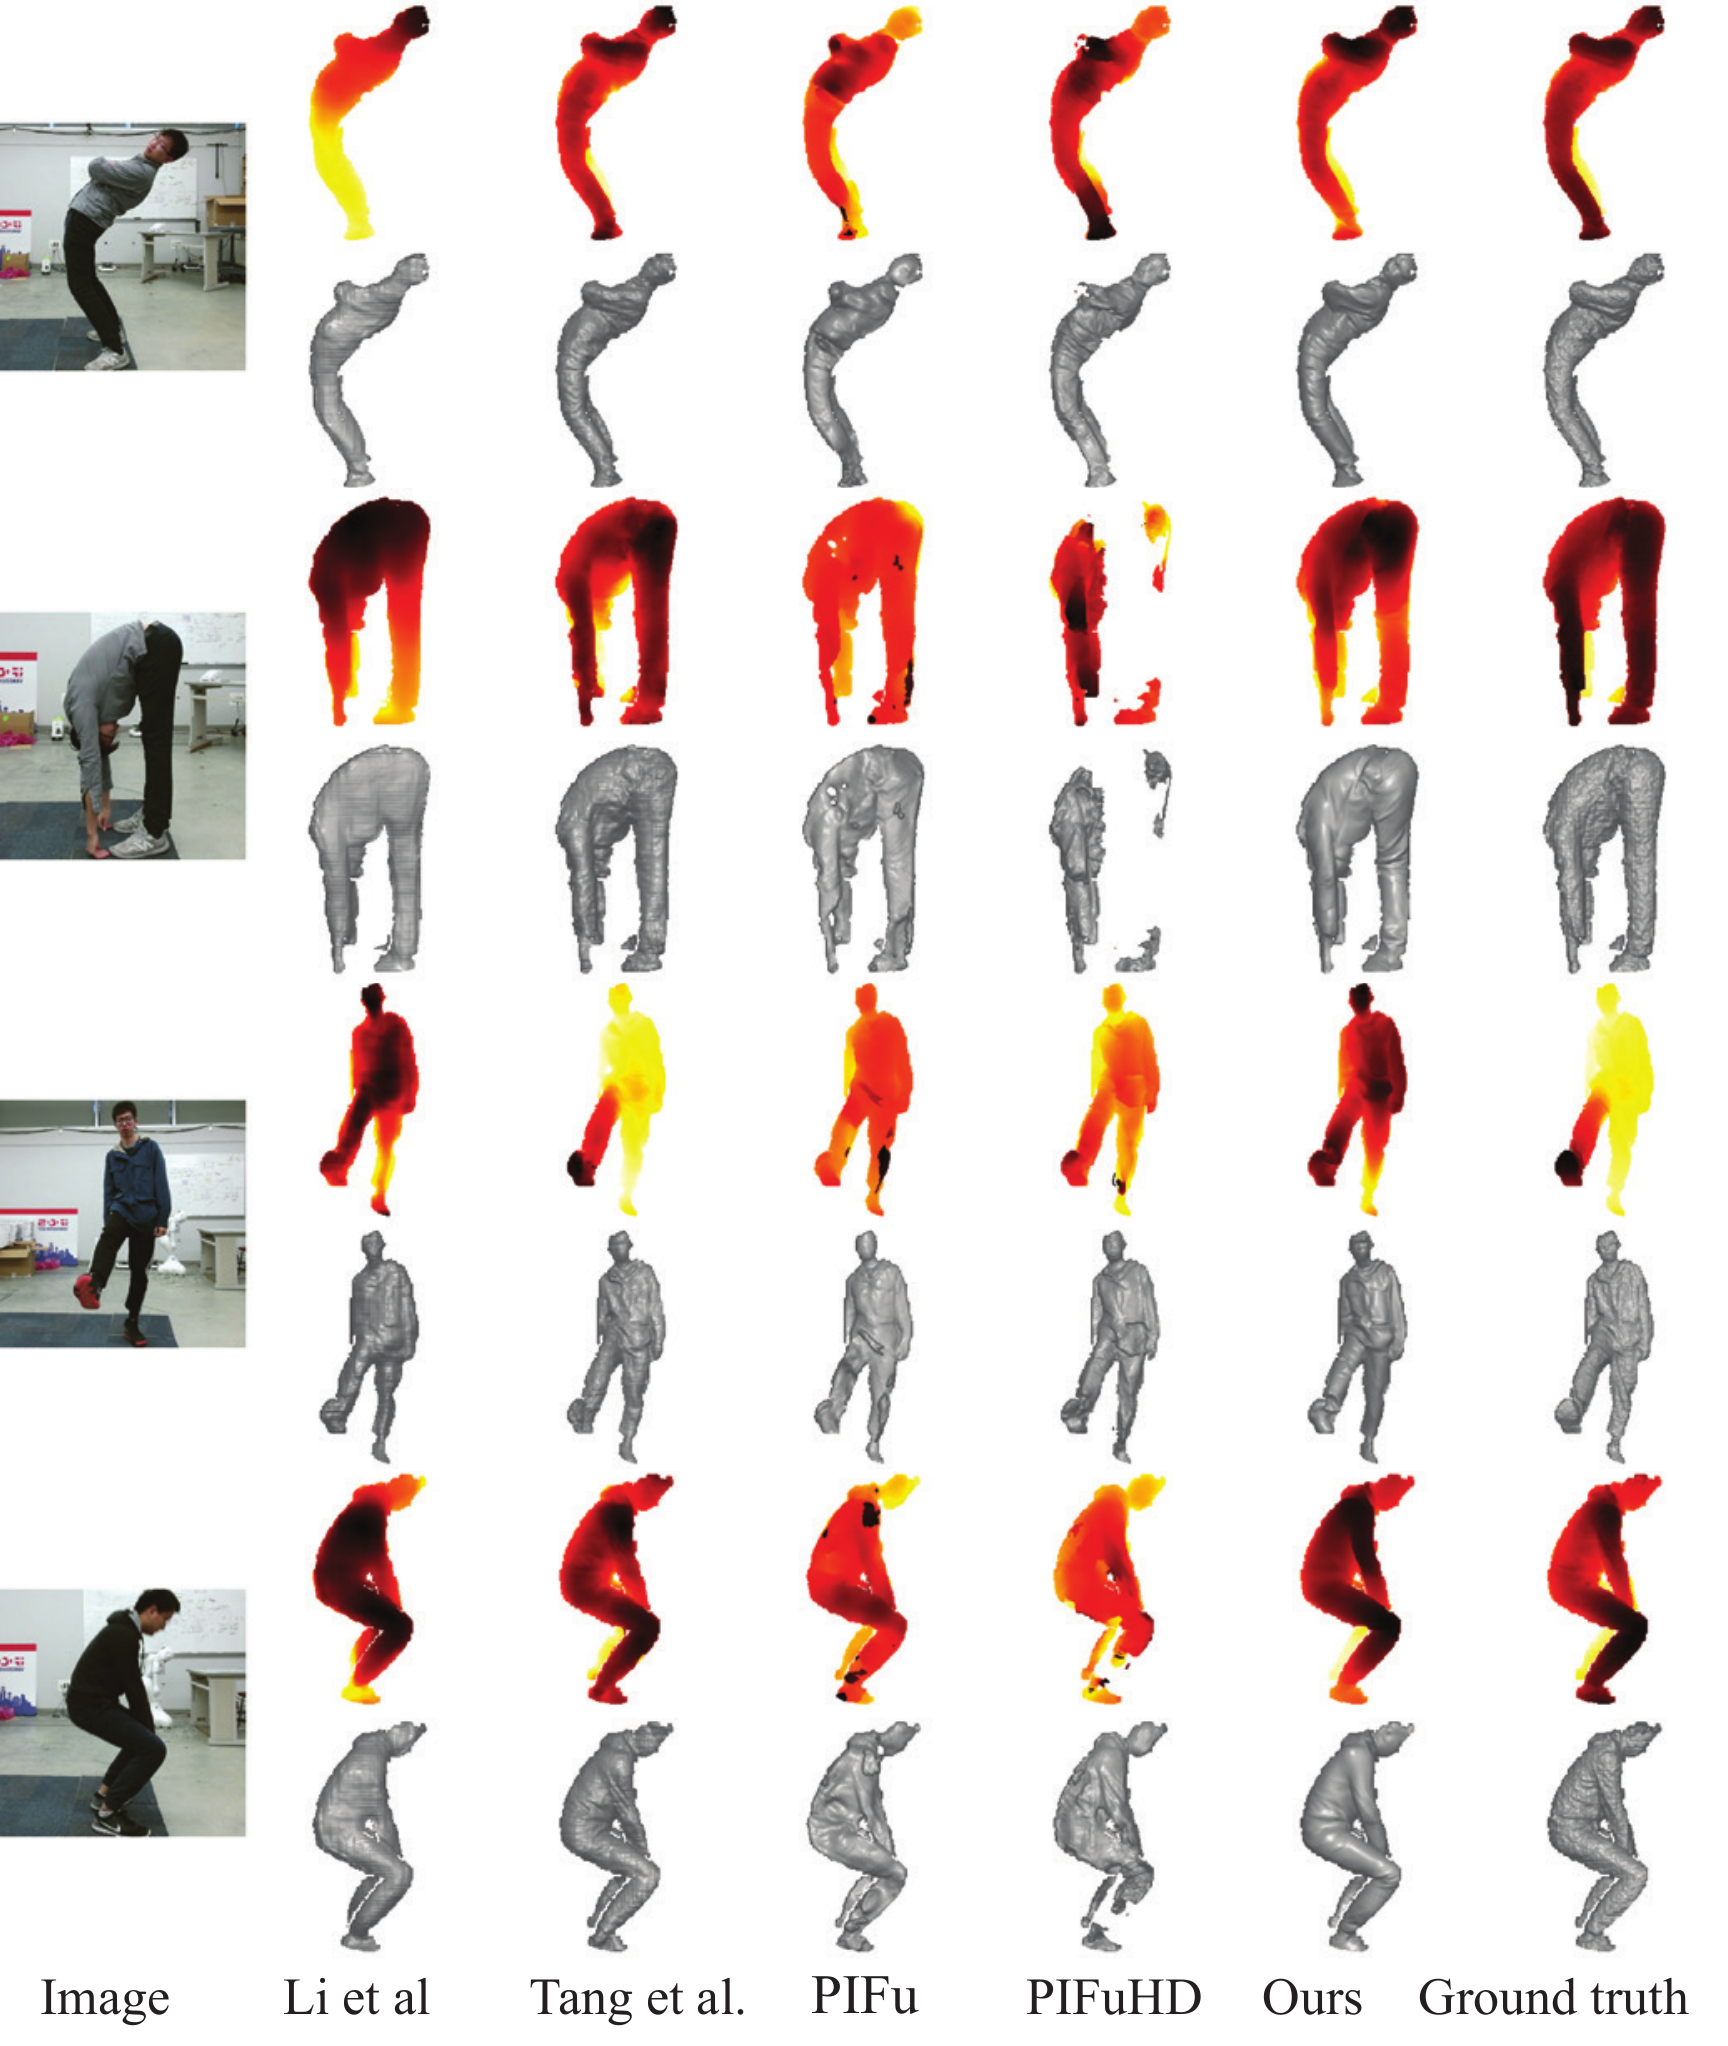}}
\end{center}
\vspace{-4mm}
   \caption{Qualitative comparison on Tang et al. training dataset}
   \label{Fig:adobe5}
\end{figure*}
